# Supplementary material for: Quantum nonlinear optics with polar J-aggregates in microcavities
Source: arXiv:1409.1930 source file (2014-09-05)
Supplement: Supplementary file 1 [file SupplementaryInfo.pdf]

# Supplementary Information for

# *Quantum nonlinear optics with polar J-aggregates in microcavities*

Felipe Herrera,[*,†] Borja Peropadre,[†] Leonardo A. Pachon,[†,‡] Semion K. Saikin,[†,¶] and Alán Aspuru-Guzik[*,†]

*Department of Chemistry and Chemical Biology, Harvard University, Cambridge, USA 02138*

E-mail: fherreraurbina@fas.harvard.edu; aspuru@chemistry.harvard.edu

[*]To whom correspondence should be addressed

[†]Department of Chemistry and Chemical Biology, Harvard University, Cambridge, USA 02138

[‡]Grupo de Física Atómica y Molecular, Instituto de Física, Facultad de Ciencias Exactas y Naturales, Universidad de Antioquia UdeA; Calle 70 No. 52-21, Medellín, Colombia.

[¶]Institute of Physics, Kazan Federal University, 18 Kremlevskaya Street, Kazan, 420008, Russian Federation

# Derivation of eq. (7) in the main text

We start with the total Hamiltonian writen in the form $\mathcal{H} = H_{\rm S} + H_{\rm SB}$. $H_{\rm S}$ describes the organic medium, the quantum fields (probe and cavity), and the light-matter interaction. $H_{\rm SB}$ describes the exciton-phonon coupling, exciton radiative decay and cavity losses through the semireflecting mirror. We assume there are $N_T$ molecules in the organic medium, forming $N_A$ identical molecular aggregates each composed of $N$ molecules ($N_T = N_A \times N$). We thus write $H_{\rm S} = \sum_{\alpha=1}^{N_A} H_{\rm S}^{\alpha}$, with a similar expansion for the system-bath coupling.

### Light-matter coupling for molecular ensemble

Following the notation in the main text, light-matter interaction Hamiltonian can be written as $H_3 = -\sum_\alpha \mathbf{D}_\alpha \mathbf{E}_\alpha$, where $\mathbf{D}_\alpha$ is the electric dipole operator of the $\alpha$-th aggregate and $\mathbf{E}_\alpha$ is the total electric field at the position of the aggregate. We assume that each aggregate experiences the same electric field to write

$$H_3 = -\sum_\alpha \mathbf{D}_\alpha \cdot \mathbf{E} \equiv -\sqrt{N_A}\mathbf{D}\cdot\mathbf{E}, \tag{1}$$

where $\mathbf{D} = (1/\sqrt{N_A}\sum_\alpha \mathbf{D}_\alpha)$ is the collective dipole operator for the molecular ensemble. The free aggregate Hamiltonian is $H_1 = \sum_\alpha H_\alpha^0 + V^\alpha$, with $H_\alpha^0 = \sum_i \epsilon_i^\alpha b_{i\alpha}^\dagger b_{i\alpha} + \sum_{ij} J_{ij}^\alpha b_{i\alpha}^\dagger b_{j\alpha}$ in the standard site-basis Frenkel exciton form,[1] and $V_\alpha$ representing exciton-exciton interaction. We write the dipole operator per aggregate $\mathbf{D}_\alpha$ in the eigenbasis $b_{k\alpha}$ of $H_0^\alpha$ as

$$\mathbf{D}_\alpha = \sum_k \mu_k^\alpha b_{k\alpha} + \sum_{kpq} \mu_{kpq}^\alpha b_{k\alpha}^\dagger b_{p\alpha} b_{q\alpha} + \text{H.c.}. \tag{2}$$

Therefore by defining the collective excitonic operators $B_k = (1/\sqrt{N_A})\sum_\alpha b_{k,\alpha}$ and $B_k^\dagger B_p B_q = (1/\sqrt{N_A})\sum_\alpha b_{k\alpha}^\dagger b_{p\alpha} b_{q\alpha}$ and expanding the quantum field $\mathbf{E}$ in terms of the probe and cavity fields we arrive at the form of $H_3$ in eq. (3) of the main text. Note that since the definition of the collective operator $B_k$ can be considered as an element of the unitary

transformation $B_k = \sum_\alpha u_{k\alpha} b_{k,\alpha}$, the operator $B_k$ have the same bosonic commutation relations as $b_{k\alpha}$. Physically, the operator $B_k^\dagger$ creates a delocalized exciton with energy $\omega_k$ in the medium, with a probability $1/N_A$ of that exciton being located in each of the aggregates in the ensemble.

### Langevin Equations

The equations of motion for the exciton and cavity photon variables are obtained from $d\hat{O}/dt = -i[O, \mathcal{H}_\mathrm{S} + \mathcal{H}_\mathrm{SB}]$, where $\hat{O}$ is a system operator. Assuming the bath degrees of freedom undergo Markovian evolution, the expectation value of the system-bath commutators of the form $\langle [\hat{O}, \mathcal{H}_\mathrm{SB}] \rangle$ lead to Langevin noise terms in the equations of motion that vanish exactly when $\hat{O}$ is linear in exciton or cavity photon operators, but can only approximately be neglected for nonlinear system operators.[2] Using the system Hamiltonian $\mathcal{H}_\mathrm{S} = H_1 + H_2 + H_3$ defined in eqs. (1)-(3) in the main text, with $V_{kp} = 2U_{kp}$, we obtain the following mean-field equations of motion

$$\frac{d}{dt}\langle B_k\rangle = -i\omega_k\langle B_k\rangle - i\sum_p V_{k,p}\langle B_p^\dagger B_p B_k\rangle - g_k\langle\mathcal{E}\rangle + \sum_{pq} D_{k,pq}\langle a^\dagger\rangle\langle B_p B_q\rangle$$
$$-2\sum_{pq} D_{q,pk}\langle a\rangle\langle B_p^\dagger B_q\rangle - i\langle[B_k,\mathcal{H}_{\mathrm{SB}}]\rangle \tag{3}$$

$$\frac{d}{dt}\langle B_p B_q\rangle = -i(\omega_p+\omega_q+V_{pq})\langle B_p B_q\rangle - \left(g_p\langle B_q\rangle + g_q\langle B_p\rangle\right)\langle\mathcal{E}\rangle$$
$$-2\sum_k D_{k,pq}\langle B_k\rangle\langle a\rangle - i\langle[B_p B_q,\mathcal{H}_{\mathrm{SB}}]\rangle \tag{4}$$

$$\frac{d}{dt}\langle B_p^\dagger B_p B_k\rangle = -i\omega_k\langle B_p^\dagger B_p B_k\rangle - i\sum_q \left(U_{kq}\langle B_p^\dagger B_q B_k\rangle + U_{pq}\langle B_p^\dagger B_q B_p\rangle\right)$$
$$-\sum_q D_{q,pk}\langle B_p^\dagger B_q\rangle\langle a\rangle - g_p\mathcal{E}^\dagger\langle B_p B_k\rangle - g_k\langle B_p^\dagger B_p\rangle\langle\mathcal{E}\rangle - g_p\langle B_k^\dagger B_k\rangle\langle\mathcal{E}\rangle$$
$$-i\langle[B_p^\dagger B_p B_k, H_{\mathrm{SB}}]\rangle \tag{5}$$

$$\frac{d}{dt}\langle B_p^\dagger B_q\rangle = -i(\omega_q-\omega_p)\langle B_p^\dagger B_q\rangle - g_p\langle\mathcal{E}^\dagger\rangle\langle B_q\rangle + g_q\langle B_q^\dagger\rangle\langle\mathcal{E}\rangle - i\langle[B_p^\dagger B_q, H_{\mathrm{SB}}]\rangle \tag{6}$$

$$\frac{d}{dt}\langle a\rangle = -i\omega_c\langle a\rangle + \sum_{kq} D_{k,kq}\langle B_k^\dagger B_k B_q\rangle - i\langle[a,\mathcal{H}_{\mathrm{SB}}]\rangle. \tag{7}$$

In the three equations above, we made a semiclassical approximation for the cavity-matter coupling in which a factorization of the form $\langle O_M O_L\rangle = \langle O_M\rangle\langle O_L\rangle$ holds, where $O_M$ represents an arbitrary material operator and $O_L$ is a cavity or probe field operator. The resulting equations are thus equivalent to the optical Bloch equation,[3] and cannot describe entanglement between the light and matter. We have also ignored the contributions deriving from the coupling to the cavity field $a$ that are proportional to the 3-point correlation function $\langle B_k^\dagger B_p B_q\rangle$. Since the probe field $\langle\mathcal{E}\rangle$ is perturbative, exciton density terms $\langle B_p^\dagger B_q\rangle$

are neglected in the steady state (see eq. (6) above). Using this fact in eq. (5) we obtain

$$\begin{aligned}\frac{d}{dt}\langle B_p^\dagger B_p B_k\rangle &= -i\omega_k\langle B_p^\dagger B_p B_k\rangle - i\sum_q \left(U_{kq}\langle B_p^\dagger B_q B_k\rangle + U_{pq}\langle B_p^\dagger B_q B_p\rangle\right)\\ &\quad -g_p\mathcal{E}^\dagger\langle B_p B_k\rangle - i\langle[B_p^\dagger B_p B_k, H_{\mathrm{SB}}]\rangle. \qquad (8)\end{aligned}$$

The one-to-two exciton coherences $\langle B_p^\dagger B_p B_k\rangle$ thus depend on the source term $g_p\mathcal{E}^\dagger\langle B_p B_k\rangle$, which scales as $|E_P|^2$ with the amplitude of the probe field. For perturbatively small $|E_p|$, as is the case for a few-photon probe field, these coherences can be neglected in the dynamical equations. Under these conditions, equations (3),(4) and (7) above give

$$\begin{aligned}\frac{d}{dt}\langle B_k\rangle &= -i\omega_k\langle B_k\rangle - g_k\langle\mathcal{E}\rangle + \sum_{pq} D_{k,pq}\langle a^\dagger\rangle\langle B_p B_q\rangle - 2\sum_{pq} D_{q,pk}\langle a\rangle\langle B_p^\dagger B_q\rangle\\ &\quad -i\langle[B_k,\mathcal{H}_{\mathrm{SB}}]\rangle \qquad (9)\\ \frac{d}{dt}\langle B_p B_q\rangle &= -i(\omega_p+\omega_q+V_{pq})\langle B_p B_q\rangle - \left(g_p\langle B_q\rangle + g_q\langle B_p\rangle\right)\langle\mathcal{E}\rangle - 2\sum_k D_{k,pq}\langle B_k\rangle\langle a\rangle\\ &\quad -i\langle[B_p B_q,\mathcal{H}_{\mathrm{SB}}]\rangle, \qquad (10)\\ \frac{d}{dt}\langle a\rangle &= -i\omega_c\langle a\rangle - i\langle[a,\mathcal{H}_{\mathrm{SB}}]\rangle \qquad (11)\end{aligned}$$

Assuming $\langle a\rangle$ is constant over the material timescales, as we do in the main text, equations (9) and (10) give eqs. (5) and (6) in the main text up to the relaxation kernels (see next section). Equation (7) in the main text follows immediately by setting the time derivatives to zero (steady state regime) and solving for the one-photon coherences $\langle B_k\rangle$.

## Relaxation Kernels

In order to account for the photon losses through the cavity mirror, radiative decay of the material into external modes and phonon scattering we need to evaluate the system-bath

commutators. We assume a bath Hamiltonian of the form $\mathcal{H}_{\rm SB} = \mathcal{H}_{\rm SB}^{(1)} + \mathcal{H}_{\rm SB}^{(2)} + \mathcal{H}_{\rm SB}^{(3)}$ with

$$\mathcal{H}_{\rm SB}^{(1)} = i\hbar \int d\omega \kappa(\omega)[b(\omega)a^\dagger - ab^\dagger(\omega)] \tag{12}$$

$$\mathcal{H}_{\rm SB}^{(2)} = i\hbar \sum_k \int d\omega \xi_k(\omega)[c_k(\omega)B_k^\dagger - B_k c_k^\dagger(\omega)] \tag{13}$$

$$\mathcal{H}_{\rm SB}^{(3)} = \sum_{pq} \int d\omega\, \lambda_{pq}(\omega)\, B_p^\dagger B_q\, [d(\omega) + d^\dagger(\omega)]. \tag{14}$$

$\mathcal{H}_{\rm SB}^{(1)}$ describes cavity decay into external electromagnetic modes represented by $b(\omega)$, $\mathcal{H}_{\rm SB}^{(2)}$ represents the radiative decay of each exciton $k$ into external modes $c_k(\omega)$, and $\mathcal{H}_{\rm SB}^{(3)}$ the scattering of excitons by phonon modes $d(\omega)$.

We briefly sketch the derivation of the relaxation tensor due to exciton-phonon scattering in the Markov approximation. For the sake of generality we rewrite eq. (14) as

$$\mathcal{H}_{\rm SB}^{(3)} = \sum_u \int d\omega K_u \otimes \Phi_u(\omega), \tag{15}$$

where we identify the system operator as $K_u \equiv B_p^\dagger B_q$ and the phonon bath operator $\Phi_u(\omega) \equiv \lambda_{pq}(\omega)[d(\omega) + d^\dagger(\omega)]$. The index $u$ runs over exciton state indices $p$ and $q$. The free bath Hamiltonian is $\mathcal{H}_{\rm B} = \int \omega d^\dagger(\omega) d(\omega) d\omega$. The Heisenberg equation for the operator $O$ is

$$\begin{aligned} \dot{O}(t) &= -i[O, \mathcal{H}_{\rm S} + \mathcal{H}_{\rm SB}^{(3)}] \\ &= -i[O, \mathcal{H}_{\rm S}] - i \sum_u \int d\omega \lambda_u(\omega)[O(t), K_u(t)]Q(\omega, t), \end{aligned} \tag{16}$$

where $Q(\omega) = d(\omega) + d^\dagger(\omega)$. Since the phonon operators evolve as

$$d(t) = \mathrm{e}^{-i\omega(t-t_0)} d(0) - i \sum_u \lambda_u(\omega) \int_{t_0}^t K_u(t'), \tag{17}$$

the phonon displacement $Q(\omega, t) = \mathrm{e}^{-i\omega(t-t_0)} d(\omega, t_0) + \mathrm{e}^{+i\omega(t-t_0)} d^\dagger(\omega, t_0) \equiv Q_\omega^{(0)}(t)$ is fully determined by the statistics of the input fields $d(\omega, t_0)$.[2] We use this fact to write a formal

solution to eq. (16) as

$$O(t) = \mathrm{e}^{-iL_{\mathrm{S}}(t-t_0)}O(t_0) - i\sum_u \int d\omega \int_{t_0}^{t} dt'\lambda_u(\omega)\left[\mathrm{e}^{-iL_{\mathrm{S}}(t-t')}O(t'), K_u(t')\right] Q_\omega^{(0)}(t'), \quad (18)$$

where $L_S O \equiv [O, \mathcal{H}_{\mathrm{S}}]$ and we take $\mathcal{H}_S = \sum_k \omega_k B_k^\dagger B_k$. Quantum Langevin equations for an arbitrary system operator can now be derived by evaluating the commutator $[O(t), K_u(t)] \equiv F(O(t))$ in the integrand of eq. (16), and inserting the formal solution in eq. (18) into $f(O(t))$. When taking the expectation values of the resulting expression over the thermal phonons, the linear term $\langle Q_\omega^{(0)}(t)\rangle$ vanishes. The bosonic correlations assume the standard form $\langle Q_\omega(t)Q_{\omega'}(t')\rangle = \delta(\omega-\omega')[(\langle n_\omega\rangle + 1)\mathrm{e}^{-i\omega(t-t')} + \langle n_\omega\rangle]\mathrm{e}^{i\omega(t-t')}]$, where $\langle n_\omega\rangle$ is the phonon thermal occupation. For $O = B_k$ we thus obtain the Langevin equation

$$\dot{B}_k = -i\omega_k B_k - \int_{t_0}^{t} dt' G_k(t-t')B_k(t'), \quad (19)$$

with a damping kernel given by

$$G_k(\tau) = \sum_q \int d\omega |\lambda_{kq}|^2 \mathrm{e}^{-i\omega_q\tau}[(\langle n_\omega\rangle + 1)\mathrm{e}^{-i\omega\tau} + \langle n_\omega\rangle]\mathrm{e}^{i\omega\tau}] \quad (20)$$

Assuming $\lambda_{kq}(\omega) \approx \lambda_{kq}$ and $\langle n_\omega\rangle \approx n(T)$ gives the Markov relaxation kernel

$$-i\langle[B_k, \mathcal{H}_{\mathrm{SB}}^{(3)}]\rangle = -\frac{\Gamma_k^\phi}{2}\langle B_k\rangle \quad (21)$$

where the phonon-induced exciton dephasing rate is $\Gamma_k^\phi = 2\sum_q |\lambda_{kq}|^2\langle n(T)\rangle$, where $k_{\mathrm{b}}T \gg \omega$ for all phonon modes. A similar derivation gives the following relaxation kernel for the two-exciton coherence in the Markov approximation

$$-i\langle[B_pB_q, \mathcal{H}_{\mathrm{SB}}^{(3)}]\rangle = -\frac{1}{2}(\Gamma_p^\phi + \Gamma_q^\phi)\langle B_pB_q\rangle \quad (22)$$

The cavity photon damping term is derived in ref.[4] using the first term in eq. (12) and

the input-output formalism. The exciton relaxation rate follows an equivalent derivation using the second term in eq. (12). The cavity damping and input terms in the Markov approximation can be written as

$$-i\langle[a(t),\mathcal{H}_{\mathrm{SB}}^{(1)}]\rangle = -\frac{\gamma_{\mathrm{c}}}{2}\langle a(t)\rangle + \sqrt{\gamma_{\mathrm{c}}}\,\langle a_{\mathrm{in}}\rangle, \tag{23}$$

where $\gamma_c$ is the decay rate of the cavity mode through the semi-reflecting mirror. When insering this expression in eq. (11), we obtain the dynamics of a damped harmonic oscillator driven by the input field $\langle a_{\mathrm{in}}\rangle$. We assume a coherent state input field field resonant with the cavity mode, in order to ensure consistency with the semiclassical approximation for the light-matter interaction and the separation of frequencies of the cavity and probe fields. In the steady-state, $\langle a\rangle$ is non-zero.

The damping term associated with the relaxation of the one and two-exciton coherences via spontaneous emission outside the cavity mode can be written in analogy with the cavity decay term as

$$-i\langle[B_k,\mathcal{H}_{\mathrm{SB}}^{(2)}]\rangle = -\frac{\gamma_k}{2}\langle B_k\rangle, \tag{24}$$

$$-i\langle[B_pB_q,\mathcal{H}_{\mathrm{SB}}^{(2)}]\rangle = -\frac{1}{2}(\gamma_p+\gamma_q)\langle B_pB_q\rangle, \tag{25}$$

where we used the fact that the photon reservoir for excitons corresponds to Gaussian noise with zero mean, i.e., $\langle B_k^{\mathrm{in}}\rangle = 0$.

Combining these results give the relaxation terms in eqs. (5) and (6) from the main text

$$\Gamma_k = \frac{1}{2}(\gamma_k+\Gamma_k^{\phi}) \tag{26}$$

$$\Gamma_{pq} = \frac{1}{2}(\gamma_k+\gamma_q+\Gamma_p^{\phi}+\Gamma_q^{\phi}). \tag{27}$$

## References

(1) Chernyak, V. and Zhang, W. M. and Mukamel, S., J. Chem. Phys. 21, 9587 (1998).

(2) Gardiner, C. W., *Quantum Noise*, Springer-Verlag (1991).

(3) Portolan, S. *et al.*, Phys. Rev. B 77, 195305 (2008).

(4) Walls, D.F. and Milburn, G. *Quantum Optics*, Springer 2nd Ed. (2008).
